# Supplementary material for: Distribution rules of systematic absence and generalized de Wolff figure of merit applied to EBSD ab-initio indexing
Source: arXiv:2003.13403 source file (2020-11-14)
Supplement: Supplementary file 1 [file supplementary.pdf]

# A Search parameters and experimental patterns used in testing the software

Table 1: Search parameters

```
# The input phi, sigma are assumed to contain errors within this range (degree).
1.0

# The unit-cell scales s1, s2 computed from the bandwidths are supposed to be equal,
# if both s1<=s2*(this.value) and s2<=s1*(this.value) hold.
3.0

# (Used only for Bravais lattice determination) squared lattice-vector lengths
# |v1|^2, |v2|^2 are supposed to be equal, if |v1|^2<=|v2|^2*(1+ this.value)
# and |v2|^2<=|v1|^2*(1+ this.value) hold.
0.05

# The number of the generated Miller indices for computing the figure of merit M.
400[a]

# The upper threshold for the absolute values |h|,|k|,|l| of the generated
# Miller indices for computing the figure of merit M.
6[a]

# Refine the projection center shift in the direction x, y, z? (No: 0, Yes: 1)
# (z-axis: perpendicular to the screen.)
1 1 1[b]

# Only the solutions with the figure of merit larger than this value is output.
3.0
```

[a]The Miller indices are generated in descending order of $d$-values.
[b]These flag was set to 1 1 0 in the analyses without using the bandwidths.

# B Simulated patterns and the parameters used for the simulation

Figures 1–3 present the band positions and widths extracted from simulated EBSD patterns and used for testing the software. The parameters used for the simulation are as follows:

Table 2: Calculation settings used by *DynamicS* software

| Sample | AV ($kV$)[a] | $d_{min}$ ($\mathring{A}$)[b] | $I_{min}$ (%)[c] | Absorption length ($\mathring{A}$)[d] | Exitation depth ($\mathring{A}$)[e] | Debye-Waller B: Crystal ($\mathring{A}^2$)[f] | Debye-Waller B: Source ($\mathring{A}^2$)[g] |
|---|---|---|---|---|---|---|---|
| $Ni$ | 20 | 0.5 | 15 | 54 | 42 | 0.74 | 0.3 |
| $Fe$ | 20 | 0.5 | 15 | 61 | 48 | 0.79 | 0.3 |
| $Zn$ | 20 | 0.5 | 15 | 68 | 54 | 0.83 | 0.3 |

[a]acceleration voltage of electron beam,
[b]minimum lattice spacing of the reflecting lattice planes,
[c]minimum intensity of a reflector relative to the strongest reflector,
[d]IMFP (Inelastic Mean Free Path) of the electrons extrapolated from the NIST Standard Reference Database,
[e]mean depth of backscattering,
[f]Debye-Waller factor of the crystal,
[g]Debye-Waller factor of the source.

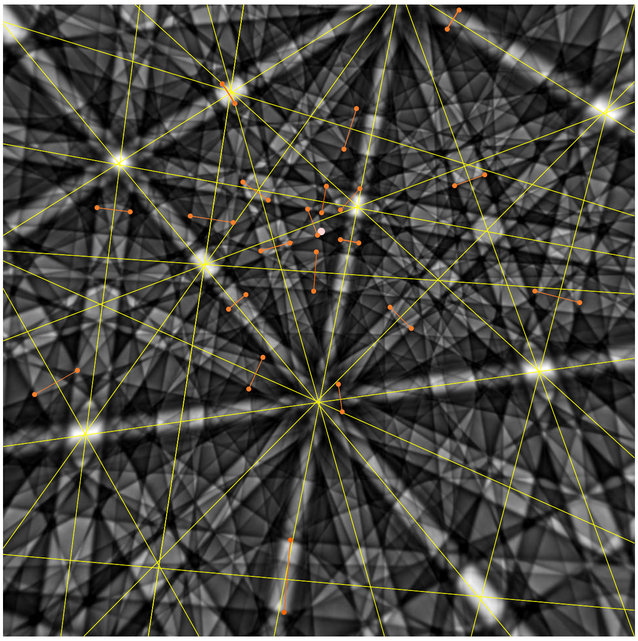

Figure 1: Band slopes and widths extracted from a simulated pattern of $Ni$ ($956 \times 956\ px^2$)

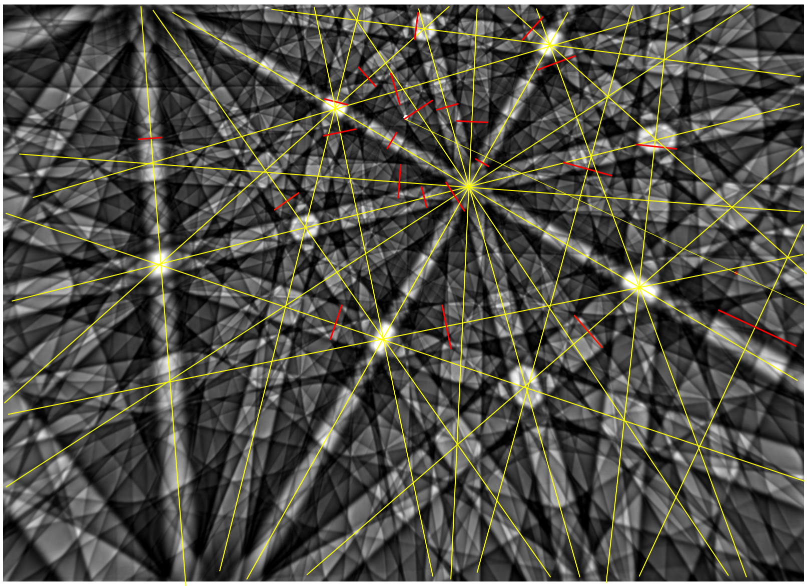

Figure 2: Band slopes and widths extracted from a simulated pattern of $Fe$ ($1600 \times 1152$ $px^2$)

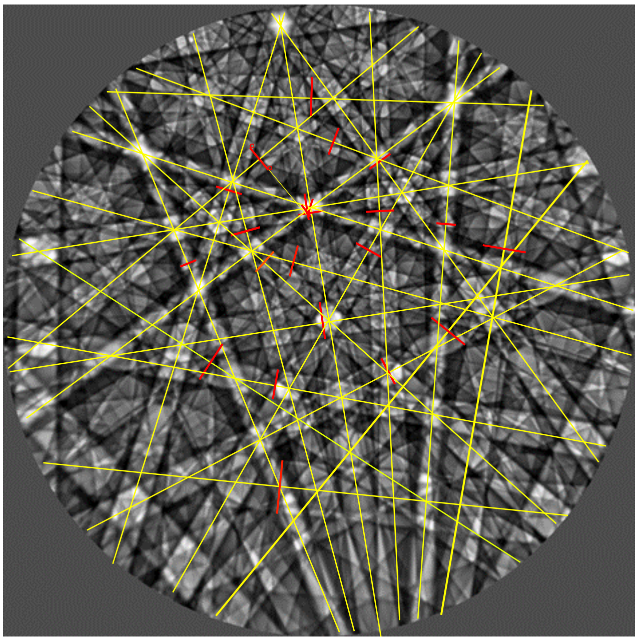

Figure 3: Band slopes and widths extracted from a simulated pattern of $Zn$ ($956 \times 956$ $px^2$)

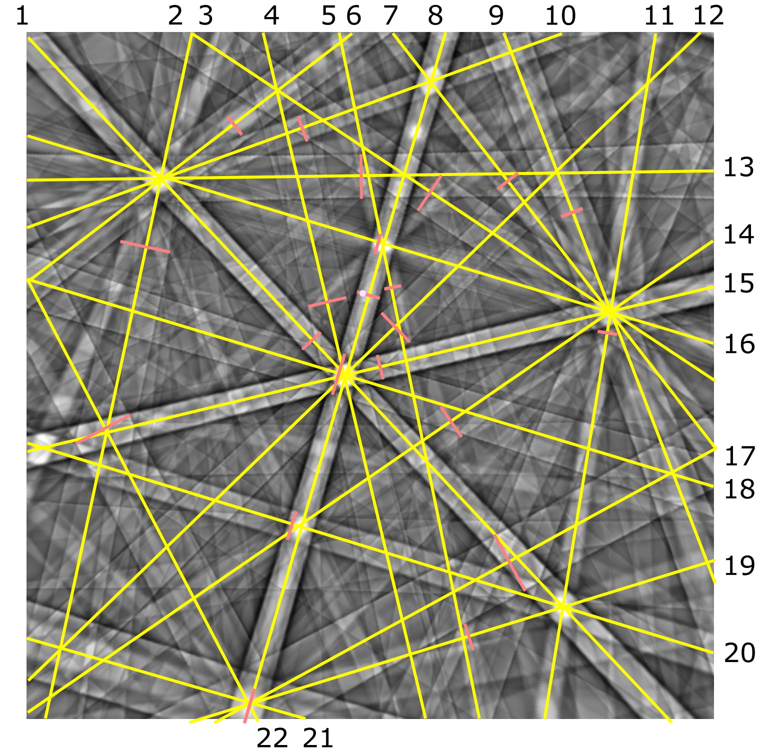


Figure 4: Band slopes and widths extracted from a simulated pattern of Silico Ferrite of $Ca$ & $Al$ ($1040 \times 1040\ px^2$)

## C De Wolff figure of merit and its generalization

As a figure of merit used for powder indexing, the de Wolff $M$ is defined as follows:

$$M_n = \bar{\epsilon}/\delta,$$

where $\bar{\epsilon}$ and $\delta$ are the *average discrepancy* and the *actual discrepancy*, respectively, defined by:

$$\bar{\epsilon} := Q_n^{obs}/2N, \tag{A.1}$$

$$\delta := \frac{1}{n}\sum_{i=1}^{n} \left|Q_i^{obs} - Q_i^{cal}\right|, \tag{A.2}$$

$$Q_i^{cal} : \text{computed line closest to the observed line } Q_i^{obs}.$$

In order to generalize the definition of $M_n$ to the sets of points in $\mathbb{R}^s$, it is important to understand why the average discrepancy is defined as (A.1), when the actual discrepancy is defined as (A.2); as explained in Wu (1988), if $q_0 := 0 < q_1 < \cdots < q_N$ is specified, the average discrepancy with regard to the $q_i$'s, is defined as:

$$\epsilon_{Wu} := \frac{1}{4q_N}\sum_{k=1}^{N}(q_k - q_{k-1})^2, \tag{A.3}$$

This $\epsilon_{Wu}$ equals to the mean value of the distance of $Q$ from its nearest $q_k$, where $Q$ is assumed to be uniformly distributed in the interval $[0, q_N]$.

If the computed lines $q_1, \ldots, q_{N-1}$ are also assumed to be uniformly distributed under the constraint $0 < q_1 < \cdots < q_{N-1} < q_N$, the mean value of $\epsilon_{Wu}$ is given by:

$$\frac{1}{4q_N}\frac{\int_0^{q_N}\cdots\int_0^{q_2}\sum_{k=1}^{N}(q_k - q_{k-1})^2 dq_1\cdots dq_{N-1}}{\int_0^{q_N}\cdots\int_0^{q_2} dq_1\cdots dq_{N-1}} = \frac{q_N}{2(N+1)}. \tag{A.4}$$

The de Wolff average discrepancy $\bar{\epsilon} := Q_n^{obs}/2N$ gives a good approximation of the formula (A.4).

In order to generalize this to a general space of dimension $s$, we consider $x_1, \ldots, x_N$ and $X_1^{obs}, \ldots, X_n^{obs}$ as points in some fixed domain $\Omega \subset \mathbb{R}^s$. In this case, it is difficult to provide a formula for the average discrepancy for the specified $x_1, \ldots, x_N$, as in (A.3). However, it is possible to estimate the mean value as in (A.4), if $x_1, \ldots, x_N$ also run over $\Omega$ with uniform probability.

Suppose that $X$ is a coordinate in $\Omega$. If $x_1, \ldots, x_{N-1}$ are uniformly distributed in $\Omega$, and $x_N$ is uniformly distributed on the boundary of $\Omega$, we have:

$$\mathrm{Prob}\left(\min_{1\le i\le N}\{|X - x_i|\} > r\right) = \left(1 - \frac{\mathrm{Vol}\,(\Omega\cap B_r(X))}{\mathrm{Vol}(\Omega)}\right)^{N-1}\left(1 - \frac{\mathrm{Area}\,(\partial\Omega\cap B_r(X))}{\mathrm{Area}(\partial\Omega)}\right).$$

where $B_r(X)$ is the ball with radius $r$ and center at $X$ of dimension $s$. $\partial\Omega$ is the surface of $\Omega$. The probability density function of $\min_{1\le i\le N}\{|X - x_i|\}$ is then given by:

$$\mathrm{Prob}\left(\min_{1\le i\le N}\{|X - x_i|\} = r\right) = -\frac{d}{dr}\mathrm{Prob}\left(\min_{1\le i\le N}\{|X - x_i|\} > r\right).$$

Hence, if $X$ is also uniformly distributed in $\Omega$, the mean value of $\min_{1\le i\le N}\{|X-x_i|\}$ is given by:

$$
\begin{aligned}
E\left[\min_{1\le i\le N}\{|X-x_i|\}\right] &= \int_0^\infty \frac{r}{\mathrm{Vol}(B_R(0))}\left(\int_{|X|\le R}\mathrm{Prob}\left(\min_{1\le i\le N}\{|X-x_i|\}=r\right)dX\right)dr \\
&= -\frac{1}{\mathrm{Vol}(B_R(0))}\int_0^\infty r\frac{d}{dr}\left(\int_{|X|\le R}\mathrm{Prob}\left(\min_{1\le i\le N}\{|X-x_i|\}>r\right)dX\right)dr \\
&= \frac{1}{\mathrm{Vol}(B_R(0))}\int_0^\infty \left(\int_{|X|\le R}\mathrm{Prob}\left(\min_{1\le i\le N}\{|X-x_i|\}>r\right)dX\right)dr \\
&= \frac{1}{\mathrm{Vol}(B_R(0))}\int_{|X|\le R}\left(\int_0^\infty \mathrm{Prob}\left(\min_{1\le i\le N}\{|X-x_i|\}>r\right)dr\right)dX.
\end{aligned}
$$

In what follows, we shall lead the formulas for the ball $\Omega=B_R(0)$ of dimension $s$.

**(Case of $s=1$)**

$$
\mathrm{Vol}\left(B_R(0)\cap B_r(X)\right) = \begin{cases} 2R & \text{if } r\ge R+|X|, \\ 2r & \text{if } r\le R-|X|, \\ r+R-|X| & \text{if } R-|X|\le r\le R+|X|. \end{cases}
$$

$$
\mathrm{Area}\left(\partial B_R(0)\cap B_r(X)\right) = \begin{cases} 2 & \text{if } r> R+|X|, \\ 0 & \text{if } r< R-|X|, \\ 1 & \text{if } R-|X|< r< R+|X|. \end{cases}
$$

Hence,

$$
\begin{aligned}
\int_0^\infty \mathrm{Prob}\left(\min_{1\le i\le N}\{|X-x_i|\}>r\right)dr &= \int_0^{R-|X|}\left(1-\frac{r}{R}\right)^{N-1}dr+\frac{1}{2}\int_{R-|X|}^{R+|X|}\left(\frac{|X|-r+R}{2R}\right)^{N-1}dr \\
&= -\frac{R}{N}\left[\left(1-\frac{r}{R}\right)^N\right]_0^{R-|X|}-\frac{R}{N}\left[\left(\frac{|X|-r+R}{2R}\right)^N\right]_{R-|X|}^{R+|X|} \\
&= -\frac{R}{N}\left\{\left(\frac{|X|}{R}\right)^N-1\right\}+\frac{R}{N}\left(\frac{|X|}{R}\right)^N=\frac{R}{N}.
\end{aligned}
$$

Therefore,

$$
E\left[\min_{1\le i\le N}\{|X-x_i|\}\right]=\frac{R}{N}=\frac{\max_{1\le i\le N}\{|x_i|\}}{N}.
$$

**(Case of $s \neq 1$)**

$$\mathrm{Vol}\left(B_R(0)\cap B_r(X)\right) = \begin{cases} \dfrac{\pi^{s/2}R^s}{\Gamma\left(\frac{s}{2}+1\right)} & \text{if } r \geq R+|X|, \\ \dfrac{\pi^{s/2}r^s}{\Gamma\left(\frac{s}{2}+1\right)} & \text{if } r \leq R-|X|, \\ \dfrac{\pi^{s/2}r^s}{\Gamma\left(\frac{s}{2}+1\right)} + \dfrac{\pi^{(s-1)/2}}{\Gamma\left(\frac{s+1}{2}\right)} \left\{ \begin{array}{l} R^s \displaystyle\int_{\frac{R^2+|X|^2-r^2}{2R|X|}}^1 (1-t^2)^{(s-1)/2}dt \\ -r^s \displaystyle\int_{\frac{R^2-|X|^2-r^2}{2r|X|}}^1 (1-t^2)^{(s-1)/2}dt \end{array} \right\} & \\ & \text{if } R-|X| \leq r \leq R+|X|. \end{cases}$$

$$\mathrm{Area}\left(\partial B_R(0)\cap B_r(X)\right) = \begin{cases} \dfrac{2\pi^{s/2}R^{s-1}}{\Gamma\left(\frac{s}{2}\right)} & \text{if } r > R+|X|, \\ 0 & \text{if } r < R-|X|, \\ \dfrac{2\pi^{(s-1)/2}R^{s-1}}{\Gamma\left(\frac{s-1}{2}\right)} \displaystyle\int_{\frac{R^2+|X|^2-r^2}{2R|X|}}^1 (1-t^2)^{(s-3)/2}dt & \text{if } R-|X| \leq r \leq R+|X|. \end{cases}$$

From geometrical considerations, we have:

$$\begin{aligned} \mathrm{Vol}\left(B_{\frac{R-|X|+r}{2}}(0)\right) < \quad & \mathrm{Vol}\left(B_R(0)\cap B_r(X)\right) & < \min\{\mathrm{Vol}\left(B_R(0)\right), \mathrm{Vol}\left(B_r(X)\right)\}, \\ 0 < \quad & \mathrm{Area}\left(\partial B_R(0)\cap B_r(X)\right) & < \min\{\mathrm{Area}\left(\partial B_R(0)\right), \mathrm{Area}\left(\partial B_r(X)\right)\}. \end{aligned}$$

Hence, we have:

$$\begin{aligned} \int_0^\infty \mathrm{Prob}_X\left(\min_{1\leq i\leq N}\{|X-x_i|\} > r\right)dr &> \int_0^{R-|X|}\left(1-\frac{r^s}{R^s}\right)^{N-1}dr \\ &\quad + \int_{R-|X|}^R \left(1-\frac{r^s}{R^s}\right)^{N-1}\left(1-\frac{r^{s-1}}{R^{s-1}}\right)dr, \\ \int_0^\infty \mathrm{Prob}_X\left(\min_{1\leq i\leq N}\{|X-x_i|\} > r\right)dr &< \int_0^{R-|X|}\left(1-\frac{r^s}{R^s}\right)^{N-1}dr \\ &\quad + \int_{R-|X|}^{R+|X|} \left(1-\frac{(R-|X|+r)^s}{2^sR^s}\right)^{N-1}dr. \end{aligned}$$

Using the variable transformations $r = Ry$ and $r_2 = Ry_2$,

$$\begin{aligned} \frac{1}{\mathrm{Vol}(B_R(0))}\int_{|X|\leq R}\left(\int_0^{R-|X|}\left(1-\frac{r^s}{R^s}\right)^{N-1}dr\right)dX &= \frac{s}{R^s}\int_0^R r_2^{s-1}\left(\int_0^{R-r_2}\left(1-\frac{r^s}{R^s}\right)^{N-1}dr\right)dr_2 \\ &= sR\int_0^1 y_2^{s-1}\left(\int_0^{1-y_2}(1-y^s)^{N-1}dy\right)dy_2 \\ &= sR\int_0^1 (1-y^s)^{N-1}\left(\int_0^{1-y} y_2^{s-1}dy_2\right)dy \\ &= R\int_0^1 (1-y^s)^{N-1}(1-y)^s dy. \end{aligned}$$

$$
\begin{aligned}
&\frac{1}{\mathrm{Vol}(B_R(0))}\int_{|X|\le R}\left(\int_{R-|X|}^{R}\left(1-\frac{r^s}{R^s}\right)^{N-1}\left(1-\frac{r^{s-1}}{R^{s-1}}\right)dr\right)dX\\
&\quad= \frac{s}{R^s}\int_0^R r_2^{s-1}\left(\int_{R-r_2}^{R}\left(1-\frac{r^s}{R^s}\right)^{N-1}\left(1-\frac{r^{s-1}}{R^{s-1}}\right)dr\right)dr_2\\
&\quad= sR\int_0^1 y_2^{s-1}\left(\int_{1-y_2}^{1}(1-y^s)^{N-1}(1-y^{s-1})dy\right)dy_2\\
&\quad= sR\int_0^1 (1-y^s)^{N-1}(1-y^{s-1})\left(\int_{1-y}^{1}y_2^{s-1}dy_2\right)dy\\
&\quad= R\int_0^1 (1-y^s)^{N-1}(1-y^{s-1})\{1-(1-y)^s\}dy.
\end{aligned}
$$

$$
\begin{aligned}
&\frac{1}{\mathrm{Vol}(B_R(0))}\int_{|X|\le R}\left(\int_{R-|X|}^{R+|X|}\left(1-\frac{(R-|X|+r)^s}{2^sR^s}\right)^{N-1}dr\right)dX\\
&\quad= \frac{s}{R^s}\int_0^R r_2^{s-1}\left(\int_{R-r_2}^{R+r_2}\left(1-\frac{(R-r_2+r)^s}{2^sR^s}\right)^{N-1}dr\right)dr_2\\
&\quad= sR\int_0^1 y_2^{s-1}\left(\int_{1-y_2}^{1+y_2}\left(1-\frac{(1-y_2+y)^s}{2^s}\right)^{N-1}dy\right)dy_2\\
&\quad= 2sR\int_0^1 y_2^{s-1}\left(\int_{1-y_2}^{1}(1-y_3^s)^{N-1}dy_3\right)dy_2 \qquad (y_3=\frac{1-y_2+y}{2})\\
&\quad= 2sR\int_0^1 (1-y_3^s)^{N-1}\left(\int_{1-y_3}^{1}y_2^{s-1}dy_2\right)dy_3 \qquad (y_3=\frac{1-y_2+y}{2})\\
&\quad= 2R\int_0^1 (1-y_3^s)^{N-1}\{1-(1-y_3)^s\}dy_3.
\end{aligned}
$$

As a result, the lower and upper bounds of $E\left[\min_{1\le i\le N}\{|X-x_i|\}\right]$ are obtained:

$$
\begin{aligned}
&E\left[\min_{1\le i\le N}\{|X-x_i|\}\right]\\
&\quad> R\int_0^1 (1-y^s)^{N-1}(1-y)^s dy + R\int_0^1 (1-y^s)^{N-1}(1-y^{s-1})\{1-(1-y)^s\}dy\\
&\quad= R\int_0^1 (1-y^s)^{N-1}\{1-y^{s-1}+y^{s-1}(1-y)^s\}dy\\
&\quad= R\int_0^1 (1-y^s)^{N-1}dy + R\sum_{k=1}^{s}\binom{s}{k}(-1)^k\int_0^1 (1-y^s)^{N-1}y^{s-1+k}dy\\
&\quad= \frac{R}{s}\int_0^1 (1-z)^{N-1}z^{(1-s)/s}dz + \frac{R}{s}\sum_{k=1}^{s}\binom{s}{k}(-1)^k\int_0^1 (1-z)^{N-1}z^{k/s}dz \qquad (z=y^s)\\
&\quad= \frac{R}{s}B(N,1/s) + \frac{R}{s}\sum_{k=1}^{s}\binom{s}{k}(-1)^k B(N,k/s+1)\\
&\quad= \frac{R}{s}\frac{\Gamma(N)\Gamma(1/s)}{\Gamma(N+1/s)} + \frac{R}{s}\sum_{k=1}^{s}\binom{s}{k}\frac{(-1)^k k}{sN+k}\frac{\Gamma(N)\Gamma(k/s)}{\Gamma(N+k/s)}.
\end{aligned}
$$

$$
\begin{aligned}
&E\left[\min_{1\le i\le N}\{|X-x_i|\}\right]\\
&\quad< \; R\int_0^1 (1-y^s)^{N-1}\{2-(1-y)^s\}dy\\
&\quad= \; R\int_0^1 (1-y^s)^{N-1}dy - R\sum_{i=1}^{s}\binom{s}{i}(-1)^i\int_0^1 (1-y^s)^{N-1}y^i dy\\
&\quad= \; \frac{R}{s}\int_0^1 (1-z)^{N-1}z^{(1-s)/s}dz - \frac{R}{s}\sum_{k=1}^{s}\binom{s}{k}(-1)^k\int_0^1 (1-z)^{N-1}z^{(1-s+k)/s}dz \qquad (z=y^s)\\
&\quad= \; \frac{R}{s}B(N,1/s) - \frac{R}{s}\sum_{k=1}^{s}\binom{s}{k}(-1)^k B(N,(k+1)/s).
\end{aligned}
$$

From $\lim_{n\to\infty}\Gamma(n)n^z/\Gamma(n+z)=1$, the beta function $B(x,y)=\Gamma(x)\Gamma(y)/\Gamma(x+y)$ has the asymptotic formula $B(x,y)\sim\Gamma(y)x^{-y}$. As a result, we have:

$$E\left[\min_{1\le i\le N}\{|X-x_i|\}\right]\sim\frac{\Gamma(1/s)}{s}\frac{R}{N^{1/s}}\quad(N\to\infty).$$

In particular, the formulas for $s=2,3$ are as follows:

**(Case of point configurations in a $2D$ ball of radius $R$)**

$$E\left[\min_{1\le i\le N}\{|X-x_i|\}\right]\sim\frac{\sqrt{\pi}}{2}\frac{R}{\sqrt{N}}\quad(N\to\infty).$$

**(Case of point configurations in a $3D$ ball of radius $R$)**

$$E\left[\min_{1\le i\le N}\{|X-x_i|\}\right]\sim\frac{\Gamma(1/3)}{3}\frac{R}{N^{1/3}}\quad(N\to\infty).$$
